# Supplementary material for: The Dark Machines Anomaly Score Challenge: Benchmark Data and Model Independent Event Classification for the Large Hadron Collider
Source: arXiv:2105.14027 source file (2021-12-09)
Supplement: Supplementary file 1 [file IndividualPhysicsModelsAppendix.tex]

\section{Results for individual physics models}
\label{app:individual}
This section shows the top 5 methods for each figure of merit for each physics signal.

\begin{figure}[h]
    \centering
    \includegraphics[width=\linewidth]{figs/IndividualSignal_chacha_cha300_neut140.pdf}
    \caption{Scores for the anomaly detection techniques on the physics signal chacha\_cha300\_neut140.}
    \label{fig:chacha300_neut140}
\end{figure}

\begin{figure}[h]
    \centering
    \includegraphics[width=\linewidth]{figs/IndividualSignal_chacha_cha400_neut60.pdf}
    \caption{Scores for the anomaly detection techniques on the physics signal chacha\_cha400\_neut60.}
    \label{fig:chacha400_neut60}
\end{figure}

\begin{figure}[h]
    \centering
    \includegraphics[width=\linewidth]{figs/IndividualSignal_chacha_cha600_neut200.pdf}
    \caption{Scores for the anomaly detection techniques on the physics signal chacha\_cha600\_neut200.}
    \label{fig:chacha600_neut200}
\end{figure}

\begin{figure}[h]
    \centering
    \includegraphics[width=\linewidth]{figs/IndividualSignal_chaneut_cha200_neut50.pdf}
    \caption{Scores for the anomaly detection techniques on the physics signal chaneut\_cha200\_neut50.}
    \label{fig:chachaneut_cha200_neut50}
\end{figure}

\begin{figure}[h]
    \centering
    \includegraphics[width=\linewidth]{figs/IndividualSignal_chaneut_cha250_neut150.pdf}
    \caption{Scores for the anomaly detection techniques on the physics signal chaneut\_cha250\_neut150.}
    \label{fig:chachaneut_cha250_neut150}
\end{figure}

\begin{figure}[h]
    \centering
    \includegraphics[width=\linewidth]{figs/IndividualSignal_chaneut_cha300_neut100.pdf}
    \caption{Scores for the anomaly detection techniques on the physics signal chaneut\_cha300\_neut100.}
    \label{fig:chachaneut_cha300_neut100}
\end{figure}

\begin{figure}[h]
    \centering
    \includegraphics[width=\linewidth]{figs/IndividualSignal_chaneut_cha400_neut200.pdf}
    \caption{Scores for the anomaly detection techniques on the physics signal chaneut\_cha400\_neut200.}
    \label{fig:chachaneut_cha400_neut200}
\end{figure}

\begin{figure}[h]
    \centering
    \includegraphics[width=\linewidth]{figs/IndividualSignal_glgl1400_neutralino1100.pdf}
    \caption{Scores for the anomaly detection techniques on the physics signal glgl1400\_neutralino1100.}
    \label{fig:glgl1400_neutralino1100}
\end{figure}

\begin{figure}[h]
    \centering
    \includegraphics[width=\linewidth]{figs/IndividualSignal_glgl1600_neutralino800.pdf}
    \caption{Scores for the anomaly detection techniques on the physics signal glgl1600\_neutralino8000.}
    \label{fig:glgl1600_neutralino800}
\end{figure}

\begin{figure}[h]
    \centering
    \includegraphics[width=\linewidth]{figs/IndividualSignal_gluino_1000.0_neutralino_1.0.pdf}
    \caption{Scores for the anomaly detection techniques on the physics signal gluino\_1000.0\_neutralino\_1.0.}
    \label{fig:gluino_1000.0_neutralino_1.0}
\end{figure}

\begin{figure}[h]
    \centering
    \includegraphics[width=\linewidth]{figs/IndividualSignal_monoV_Zp2000.0_DM_1.0.pdf}
    \caption{Scores for the anomaly detection techniques on the physics signal monoV\_Zp2000.0\_DM\_1.0.}
    \label{fig:monoV_Zp2000.0_DM_1.0}
\end{figure}

\begin{figure}[h]
    \centering
    \includegraphics[width=\linewidth]{figs/IndividualSignal_monojet_Zp2000.0_DM_50.0.pdf}
    \caption{Scores for the anomaly detection techniques on the physics signal monojet\_Zp2000.0\_DM\_50.0.}
    \label{fig:monojet_Zp2000.0_DM_50.0}
\end{figure}

\begin{figure}[h]
    \centering
    \includegraphics[width=\linewidth]{figs/IndividualSignal_monotop_200_A.pdf}
    \caption{Scores for the anomaly detection techniques on the physics signal monotop\_200\_A.}
    \label{fig:monotop_200_A}
\end{figure}

\begin{figure}[h]
    \centering
    \includegraphics[width=\linewidth]{figs/IndividualSignal_pp23mt_50.pdf}
    \caption{Scores for the anomaly detection techniques on the physics signal pp23mt\_50.}
    \label{fig:mpp23mt_50}
\end{figure}

\begin{figure}[h]
    \centering
    \includegraphics[width=\linewidth]{figs/IndividualSignal_pp24mt_50.pdf}
    \caption{Scores for the anomaly detection techniques on the physics signal pp24mt\_50.}
    \label{fig:pp24mt_50}
\end{figure}

\begin{figure}[h]
    \centering
    \includegraphics[width=\linewidth]{figs/IndividualSignal_sqsq1_sq1400_neut800.pdf}
    \caption{Scores for the anomaly detection techniques on the physics signal sqsq1\_sq1400\_neut800.}
    \label{fig:sqsq1_sq1400_neut800}
\end{figure}

\begin{figure}[h]
    \centering
    \includegraphics[width=\linewidth]{figs/IndividualSignal_sqsq1_sq1400_neut800.pdf}
    \caption{Scores for the anomaly detection techniques on the physics signal sqsq1\_sq1400\_neut800.}
    \label{fig:sqsq1_sq1400_neut800}
\end{figure}

\begin{figure}[h]
    \centering
    \includegraphics[width=\linewidth]{figs/IndividualSignal_stlp_st1000.pdf}
    \caption{Scores for the anomaly detection techniques on the physics signal stlp\_st1000.}
    \label{fig:stlp_st1000}
\end{figure}

\begin{figure}[h]
    \centering
    \includegraphics[width=\linewidth]{figs/IndividualSignal_stop2b1000_neutralino300.pdf}
    \caption{Scores for the anomaly detection techniques on the physics signal stop2b1000\_neutralino300.}
    \label{fig:stop2b1000_neutralino300}
\end{figure}
